# Supplementary material for: Test-Time Adaptation with Perturbation Consistency Learning
Source: arXiv:2304.12764 source file (2023-04-25)
Supplement: Supplementary file 1 [file appendix-detail.tex]

\begin{table*}[htb]
\centering
\caption{Detailed results (\%) on NoiseQA-syn.}
\vskip 0.15in
%\small
%\resizebox{\textwidth}{!}{
    \begin{tabular}{l c c c c c c c c c c c }
    \toprule
\multirow{2}{*}{\textbf{Models}} & \multicolumn{2}{c}{\textbf{asr}} & \multicolumn{2}{c}{\textbf{keyboard}} & \multicolumn{2}{c}{\textbf{translation}}& \multicolumn{2}{c}{\textbf{avg}}\\
\cmidrule(r){2-3} \cmidrule(r){4-5} \cmidrule(r){6-7} \cmidrule(r){8-9}
 &\textbf{EM} & \textbf{F1} & \textbf{EM} &\textbf{F1} & \textbf{EM} & \textbf{F1} & \textbf{EM} & \textbf{F1}\\
    \midrule
    xlmr-base & 67.14 & 79.95 & 64.71 & 76.29 & 67.98 & 79.66 & 66.64 & 78.67\\
    xTune & 71.51 & 82.62 & 70.08 & 80.02 & 71.18 & 81.83 & 70.95 & 81.52\\
    \midrule
    Tent & 67.20 & 78.90 & 63.47 & 74.51 & 66.16 & 77.78 & 65.61 & 77.06\\
    EATA & 66.92 & 78.67 & 62.86 & 73.95 & 65.91 & 77.58 & 65.23 & 76.73\\
    OIL & 69.83 & 81.28 & 66.81 & 77.50 & 69.02 & 80.18 & 68.55 & 79.65\\
    PCL & 70.06 & 81.53 & 66.39 & 77.24 & 68.88 & 80.07 & 68.44 & 79.61\\
    \midrule
    xTune+Tent & 71.18 & 81.95 & 69.58 & 79.75 & 70.00 & 80.70 & 70.25 & 80.80\\
    xTune+EATA & 70.78 & 81.58 & 69.22 & 79.36 & 69.50 & 80.33 & 69.83 & 80.42\\
    xTune+OIL & 72.35 & 82.85 & 71.32 & 81.03 & 70.86 & 81.58 & 71.51 & 81.82\\
    xTune+PCL & 72.16 & 82.77 & 71.51 & 81.09 & 70.90 & 81.77 & 71.52 & 81.88\\
    \midrule
    \midrule
    xlmr-large & 53.45 & 72.47 & 72.94 & 84.66 & 70.25 & 82.60 & 65.55 & 79.91 \\
    xTune & 58.57 & 75.83 & 76.47 & 87.36 & 75.29 & 86.32 & 70.11 & 83.17\\
    \midrule
    Tent & 71.34 & 83.37 & 72.02 & 83.49 & 69.89 & 82.07 & 71.08 & 82.97\\
    EATA & 71.88 & 83.69 & 72.30 & 83.49 & 69.41 & 81.62 & 71.20 & 82.93\\
    OIL & 69.83 & 83.43 & 73.22 & 85.01 & 70.06 & 82.61 & 71.03 & 83.68\\
    PCL & 71.48 & 83.99 & 73.33 & 84.57 & 70.76 & 82.69 & 71.86 & 83.75\\
    \midrule
    xTune+Tent & 75.77 & 86.52 & 76.41 & 86.84 & 74.99 & 85.60 & 75.72 & 86.32\\
    xTune+EATA & 75.63 & 86.40 & 76.39 & 86.68 & 74.68 & 85.29 & 75.56 & 86.12\\
    xTune+OIL & 75.69 & 86.79 & 76.81 & 87.25 & 75.32 & 86.13 & 75.94 & 86.72\\
    xTune+PCL & 75.85 & 86.69 & 76.83 & 87.22 & 75.63 & 86.18 & 76.11 & 86.69\\
    \bottomrule
    \end{tabular}
%}
\vskip -0.1in
\end{table*}

\begin{table*}[htb]
\centering
\caption{Detailed results (\%) on NoiseQA-na.}
\vskip 0.15in
%\small
%\resizebox{\textwidth}{!}{
    \begin{tabular}{l c c c c c c c c c c c }
    \toprule
\multirow{2}{*}{\textbf{Models}} & \multicolumn{2}{c}{\textbf{asr}} & \multicolumn{2}{c}{\textbf{keyboard}} & \multicolumn{2}{c}{\textbf{translation}}& \multicolumn{2}{c}{\textbf{avg}}\\
\cmidrule(r){2-3} \cmidrule(r){4-5} \cmidrule(r){6-7} \cmidrule(r){8-9}
 &\textbf{EM} & \textbf{F1} & \textbf{EM} &\textbf{F1} & \textbf{EM} & \textbf{F1} & \textbf{EM} & \textbf{F1}\\
    \midrule
    xlmr-base & 57.98 & 70.79 & 71.01 & 82.41 & 69.24 & 80.56 & 66.25 & 77.91\\
    xTune & 63.78 & 75.16 & 73.95 & 84.59 & 71.43 & 82.20 & 69.75 & 80.66\\
    \midrule
    Tent & 59.33 & 70.65 & 68.96 & 80.37 & 66.89 & 78.12 & 65.06 & 76.38\\
    EATA & 58.68 & 69.89 & 68.68 & 80.33 & 66.58 & 77.92 & 64.65 & 76.05\\
    OIL & 63.56 & 74.43 & 70.81 & 82.28 & 68.88 & 80.11 & 67.75 & 78.94\\
    PCL & 62.27 & 73.52 & 71.43 & 82.74 & 68.52 & 79.82 & 67.40 & 78.69\\
    \midrule
    xTune+Tent & 65.35 & 74.75 & 73.53 & 83.87 & 70.67 & 81.51 & 69.85 & 80.04\\
    xTune+EATA & 65.04 & 74.59 & 73.08 & 83.64 & 70.31 & 81.19 & 69.48 & 79.81\\
    xTune+OIL & 65.85 & 75.98 & 73.92 & 84.35 & 71.29 & 81.96 & 70.35 & 80.76\\
    xTune+PCL & 66.27 & 76.40 & 74.23 & 84.82 & 71.54 & 82.24 & 70.68 & 81.15\\
    \midrule
    \midrule
    xlmr-large & 46.13 & 64.62 & 73.53 & 85.86 & 72.86 & 84.63 & 64.17 & 78.37 \\
    xTune & 49.41 & 66.78 & 76.47 & 88.12 & 75.71 & 86.72 & 67.20 & 80.54\\
    \midrule
    Tent & 61.18 & 73.76 & 73.75 & 85.40 & 70.78 & 82.80 & 68.57 & 80.65\\
    EATA & 61.71 & 73.92 & 73.47 & 85.15 & 71.12 & 82.76 & 68.77 & 80.61\\
    OIL & 61.18 & 74.78 & 74.65 & 86.26 & 72.94 & 84.52 & 69.59 & 81.85\\
    PCL & 61.88 & 74.96 & 73.98 & 86.22 & 73.33 & 84.53 & 69.73 & 81.90\\
    \midrule
    xTune+Tent & 66.81 & 77.64 & 77.87 & 88.05 & 75.43 & 86.10 & 73.37 & 83.93\\
    xTune+EATA & 66.89 & 77.92 & 77.31 & 87.73 & 75.41 & 85.98 & 73.20 & 83.88\\
    xTune+OIL & 66.81 & 78.32 & 77.54 & 88.31 & 76.22 & 86.81 & 73.52 & 84.48\\
    xTune+PCL & 67.70 & 78.38 & 77.82 & 88.51 & 76.16 & 86.85 & 73.89 & 84.58\\
    \bottomrule
    \end{tabular}
%}
\vskip -0.1in
\end{table*}

\begin{table*}[htb]
\centering
\caption{Detailed results (\%) on XQuAD (EM).}
\vskip 0.15in
%\small
%\resizebox{\textwidth}{!}{
    \begin{tabular}{l c c c c c c c c c c c c}
    \toprule
\textbf{Models} & en & es & de & el & ru & tr & ar & vi & th & zh & hi & \textbf{avg} \\
    \midrule
    xlmr-base & 72.52 & 58.07 & 58.15 & 54.54 & 57.56 & 50.92 & 48.99 & 55.38 & 55.13 & 51.60 & 48.66 & 55.59\\
    xTune & 74.71 & 60.67 & 62.52 & 58.15 & 61.18 & 54.29 & 52.02 & 55.21 & 59.83 & 53.87 & 54.45 & 58.81\\
    \midrule
   Tent & 70.00 & 56.50 & 54.54 & 53.45 & 54.57 & 47.42 & 45.69 & 52.16 & 54.45 & 54.54 & 48.24 & 53.78\\
    EATA & 69.69 & 56.22 & 54.79 & 53.47 & 54.34 & 48.24 & 44.59 & 51.68 & 57.14 & 55.18 & 48.10 & 53.95\\
    OIL & 72.18 & 60.00 & 58.26 & 56.19 & 57.48 & 51.99 & 48.88 & 55.18 & 62.61 & 59.72 & 51.43 & 57.63\\
    PCL & 72.68 & 59.18 & 58.03 & 56.10 & 58.09 & 52.37 & 49.43 & 55.29 & 57.82 & 55.73 & 51.27 & 56.91\\
    \midrule
    xTune+Tent & 73.89 & 60.11 & 60.06 & 57.06 & 58.66 & 52.89 & 49.61 & 54.65 & 59.80 & 55.21 & 53.19 & 57.74\\
    xTune+EATA & 73.64 & 59.36 & 59.41 & 56.61 & 58.26 & 52.66 & 49.44 & 54.34 & 60.00 & 56.08 & 53.11 & 57.54\\
    xTune+OIL & 73.89 & 61.23 & 62.55 & 59.50 & 60.17 & 55.71 & 52.16 & 57.28 & 63.70 & 57.28 & 54.96 & 59.86\\
    xTune+PCL & 74.87 & 61.23 & 62.24 & 59.05 & 60.53 & 55.49 & 52.30 & 56.89 & 62.32 & 56.78 & 54.73 & 59.68\\
    \midrule
    \midrule
    xlmr-large & 75.38 & 63.87 & 62.52 & 63.78 & 63.53 & 59.92 & 58.57 & 61.60 & 64.62 & 61.51 & 59.33 & 63.15\\
    xTune & 77.82 & 65.80 & 67.31 & 66.47 & 65.71 & 61.68 & 60.50 & 63.28 & 63.78 & 59.41 & 63.28 & 65.00\\
    \midrule
    Tent & 74.17 & 62.66 & 62.13 & 61.04 & 61.65 & 57.90 & 57.28 & 59.02 & 65.46 & 65.57 & 58.10 & 62.27\\
    EATA & 73.98 & 62.77 & 62.18 & 61.12 & 61.76 & 58.10 & 56.72 & 58.85 & 65.94 & 66.13 & 57.96 & 62.32\\
    OIL & 75.91 & 63.78 & 62.72 & 62.61 & 63.64 & 59.86 & 58.66 & 61.26 & 68.99 & 68.74 & 60.53 & 64.24\\
    PCL & 75.63 & 64.03 & 62.63 & 63.84 & 63.64 & 59.86 & 58.71 & 60.92 & 66.64 & 65.69 & 60.22 & 63.80\\
    \midrule
    xTune+Tent & 78.04 & 66.41 & 66.69 & 65.15 & 64.59 & 61.74 & 60.20 & 62.94 & 67.11 & 61.85 & 62.77 & 65.23\\
    xTune+EATA & 77.62 & 66.08 & 66.50 & 64.51 & 64.31 & 61.29 & 59.94 & 62.41 & 67.31 & 61.85 & 62.61 & 64.95\\
    xTune+OIL & 78.32 & 67.14 & 68.21 & 65.85 & 65.32 & 62.13 & 60.64 & 63.89 & 68.21 & 63.31 & 63.22 & 66.02\\
    xTune+PCL & 78.35 & 67.00 & 66.92 & 66.30 & 65.10 & 62.18 & 60.76 & 64.15 & 67.31 & 62.46 & 63.42 & 65.81\\
    \bottomrule
    \end{tabular}
%}
\vskip -0.1in
\end{table*}

\begin{table*}[htb]
\centering
\caption{Detailed results (\%) on XQuAD (F1).}
\vskip 0.15in
%\small
%\resizebox{\textwidth}{!}{
    \begin{tabular}{l c c c c c c c c c c c c}
    \toprule
\textbf{Models} & en & es & de & el & ru & tr & ar & vi & th & zh & hi & \textbf{avg} \\
    \midrule
    xlmr-base & 83.73 & 76.71 & 74.56 & 72.56 & 74.30 & 67.88 & 66.06 & 73.80 & 66.38 & 63.52 & 66.23 & 71.43\\
    xTune & 85.14 & 77.76 & 77.80 & 75.69 & 76.62 & 70.54 & 69.05 & 74.92 & 68.91 & 64.14 & 70.90 & 73.77\\
    \midrule
    Tent & 81.49 & 74.37 & 70.31 & 69.70 & 71.30 & 63.56 & 62.86 & 71.76 & 64.82 & 64.95 & 63.42 & 68.96\\
    EATA & 81.23 & 73.93 & 70.22 & 69.62 & 71.02 & 63.72 & 62.02 & 71.24 & 67.06 & 64.38 & 62.91 & 68.85\\
    OIL & 83.41 & 77.31 & 73.91 & 72.42 & 74.04 & 67.76 & 65.92 & 73.81 & 71.58 & 68.61 & 67.30 & 72.37\\
    PCL & 83.78 & 76.77 & 74.41 & 72.45 & 74.48 & 68.20 & 66.27 & 73.79 & 68.22 & 65.91 & 66.98 & 71.93\\
    \midrule
    xTune+Tent & 84.30 & 76.72 & 74.68 & 73.40 & 74.53 & 68.22 & 66.74 & 74.28 & 68.36 & 64.12 & 68.52 & 72.17\\
    xTune+EATA & 84.10 & 75.89 & 74.31 & 72.85 & 74.25 & 67.87 & 66.46 & 74.02 & 68.28 & 64.49 & 68.39 & 71.90\\
    xTune+OIL & 84.72 & 77.79 & 77.33 & 75.40 & 76.06 & 71.49 & 69.44 & 76.43 & 72.02 & 66.24 & 71.21 & 74.38\\
    xTune+PCL & 85.21 & 77.39 & 77.08 & 75.54 & 76.10 & 70.41 & 69.63 & 75.91 & 70.76 & 65.65 & 70.99 & 74.06\\
    \midrule
    \midrule
    xlmr-large & 86.96 & 82.57 & 80.20 & 81.27 & 79.75 & 76.58 & 75.71 & 80.73 & 75.26 & 71.02 & 76.45 & 78.77\\
    xTune & 88.96 & 83.56 & 83.26 & 82.64 & 82.08 & 77.29 & 77.51 & 82.47 & 73.62 & 68.67 & 78.92 & 79.91\\
    \midrule
    Tent & 85.95 & 81.00 & 79.27 & 79.09 & 78.61 & 74.75 & 74.23 & 78.76 & 75.41 & 73.70 & 74.66 & 77.77\\
    EATA & 85.79 & 80.73 & 79.12 & 78.71 & 78.67 & 74.51 & 73.66 & 78.52 & 75.55 & 73.96 & 74.22 & 77.59\\
    OIL & 87.03 & 82.43 & 79.81 & 80.49 & 80.43 & 76.13 & 75.70 & 80.41 & 77.89 & 76.24 & 76.89 & 79.40\\
    PCL & 86.97 & 82.15 & 79.90 & 80.76 & 80.01 & 76.09 & 75.69 & 80.14 & 76.60 & 73.94 & 76.45 & 78.97\\
    \midrule
    xTune+Tent & 88.46 & 82.90 & 82.44 & 81.81 & 81.04 & 77.02 & 76.65 & 81.71 & 75.81 & 69.51 & 78.05 & 79.58\\
    xTune+EATA & 88.27 & 82.47 & 82.13 & 81.17 & 80.77 & 76.72 & 76.43 & 81.43 & 75.58 & 69.22 & 77.85 & 79.28\\
    xTune+OIL & 89.05 & 83.72 & 83.27 & 82.32 & 81.62 & 77.45 & 77.34 & 82.61 & 76.61 & 70.69 & 79.07 & 80.34\\
    xTune+PCL & 88.79 & 83.40 & 82.85 & 82.39 & 81.50 & 77.46 & 77.44 & 82.54 & 75.62 & 70.04 & 78.80 & 80.08\\
    \bottomrule
    \end{tabular}
%}
\vskip -0.1in
\end{table*}

\begin{table*}[htb]
\centering
\caption{Detailed results (\%) on MLQA (EM).}
\vskip 0.15in
%\small
%\resizebox{\textwidth}{!}{
    \begin{tabular}{l c c c c c c c c c c c c}
    \toprule
    \textbf{Models} & en & es & de & ar & hi & vi & zh & \textbf{avg} \\
    \midrule
    xlmr-base & 67.58 & 50.20 & 47.93 & 38.20 & 42.90 & 46.28 & 36.77 & 47.12\\
    xTune & 69.13 & 51.84 & 50.52 & 39.23 & 47.25 & 48.86 & 42.24 & 49.87\\
    \midrule
    Tent & 65.06 & 47.24 & 45.49 & 34.12 & 39.81 & 43.72 & 33.85 & 44.18\\
    EATA & 64.84 & 47.26 & 45.30 & 33.71 & 39.47 & 43.31 & 33.99 & 43.98\\
    OIL & 68.08 & 50.23 & 48.22 & 38.51 & 44.29 & 47.15 & 38.81 & 47.90\\
    PCL & 67.72 & 50.16 & 48.16 & 38.16 & 43.62 & 46.44 & 37.38 & 47.38\\
    \midrule
    xTune+Tent & 68.61 & 50.54 & 48.65 & 37.49 & 44.52 & 47.19 & 40.39 & 48.20\\
    xTune+EATA & 68.37 & 50.50 & 48.69 & 36.91 & 43.89 & 46.99 & 40.45 & 47.97\\
    xTune+OIL & 69.70 & 52.08 & 50.47 & 40.60 & 48.55 & 49.07 & 42.81 & 50.47\\
    xTune+PCL & 69.44 & 52.12 & 50.68 & 39.51 & 47.55 & 48.90 & 42.45 & 50.09\\
    \midrule
    \midrule
    xlmr-large & 70.14 & 56.33 & 55.88 & 46.56 & 52.75 & 52.59 & 42.87 & 53.87\\
    xTune & 72.89 & 58.04 & 56.87 & 48.12 & 55.41 & 54.47 & 48.32 & 56.30\\
    \midrule
    Tent & 69.57 & 54.74 & 53.99 & 43.77 & 50.47 & 51.36 & 41.42 & 52.19\\
    EATA & 69.49 & 54.69 & 53.91 & 43.76 & 50.37 & 51.20 & 41.59 & 52.15\\
    OIL & 70.71 & 56.42 & 55.91 & 46.57 & 52.56 & 52.59 & 44.59 & 54.19\\
    PCL & 70.53 & 56.41 & 55.79 & 46.68 & 52.56 & 52.58 & 43.48 & 54.00\\
    \midrule
    xTune+Tent & 72.68 & 57.02 & 56.42 & 46.83 & 54.03 & 53.59 & 47.19 & 55.39\\
    xTune+EATA & 72.62 & 56.98 & 56.50 & 46.70 & 53.96 & 53.56 & 47.17 & 55.36\\
    xTune+OIL & 73.05 & 57.74 & 57.07 & 47.98 & 55.22 & 54.32 & 48.08 & 56.21\\
    xTune+PCL & 73.12 & 57.84 & 56.93 & 48.04 & 55.52 & 54.34 & 48.26 & 56.29\\
    \bottomrule
    \end{tabular}
%}
\vskip -0.1in
\end{table*}

\begin{table*}[htb]
\centering
\caption{Detailed results (\%) on MLQA (F1).}
\vskip 0.15in
%\small
%\resizebox{\textwidth}{!}{
    \begin{tabular}{l c c c c c c c c c c c c}
    \toprule
\textbf{Models} & en & es & de & ar & hi & vi & zh & \textbf{avg} \\
    \midrule
    xlmr-base & 80.45 & 67.68 & 62.53 & 57.12 & 61.02 & 67.06 & 61.01 & 65.27\\
    xTune & 81.75 & 69.56 & 65.41 & 59.03 & 64.37 & 69.62 & 64.54 & 67.76\\
    \midrule
    Tent & 78.15 & 64.97 & 60.29 & 52.97 & 57.46 & 64.28 & 57.98 & 62.30\\
    EATA & 77.90 & 64.87 & 60.07 & 52.53 & 56.94 & 63.85 & 58.01 & 62.02\\
    OIL & 80.62 & 67.54 & 62.46 & 57.23 & 61.43 & 67.48 & 62.03 & 65.54\\
    PCL & 80.40 & 67.36 & 62.49 & 56.98 & 61.07 & 66.95 & 61.33 & 65.23\\
    \midrule
    xTune+Tent & 80.93 & 68.05 & 63.54 & 56.61 & 61.21 & 67.70 & 62.77 & 65.83\\
    xTune+EATA & 80.70 & 67.96 & 63.58 & 55.95 & 60.44 & 67.41 & 62.83 & 65.55\\
    xTune+OIL & 82.04 & 69.58 & 65.25 & 60.14 & 65.37 & 69.89 & 65.18 & 68.21\\
    xTune+PCL & 81.73 & 69.69 & 65.43 & 59.29 & 64.22 & 69.58 & 64.67 & 67.80\\
    \midrule
    \midrule
    xlmr-large & 83.46 & 74.63 & 70.68 & 66.74 & 70.85 & 74.00 & 67.67 & 72.58\\
    xTune & 85.40 & 75.57 & 71.82 & 67.89 & 73.05 & 75.79 & 70.78 & 74.33\\
    \midrule
    Tent & 82.74 & 73.04 & 69.16 & 64.19 & 68.34 & 72.85 & 66.27 & 70.94\\
    EATA & 82.66 & 72.96 & 69.02 & 64.06 & 68.20 & 72.74 & 66.32 & 70.85\\
    OIL & 83.76 & 74.60 & 70.56 & 66.73 & 70.91 & 74.01 & 68.48 & 72.72\\
    PCL & 83.60 & 74.58 & 70.47 & 66.73 & 70.71 & 73.92 & 67.95 & 72.56\\
    \midrule
    xTune+Tent & 85.00 & 74.79 & 71.17 & 66.84 & 71.79 & 74.97 & 69.97 & 73.50\\
    xTune+EATA & 84.90 & 74.70 & 71.17 & 66.61 & 71.71 & 74.88 & 69.95 & 73.42\\
    xTune+OIL & 85.45 & 75.41 & 71.89 & 67.67 & 73.00 & 75.63 & 70.59 & 74.23\\
    xTune+PCL & 85.44 & 75.47 & 71.81 & 67.74 & 73.08 & 75.63 & 70.72 & 74.27\\
    \bottomrule
    \end{tabular}
%}
\vskip -0.1in
\end{table*}
